# Supplementary material for: Refined Inference for Asymptotically Linear Estimators with Non-Negligible Second-Order Remainders
Source: arXiv:2603.16833 source file (2026-11-16)
Supplement: Supplementary file 1 [file supplement.tex]

% ============================================================
%  Supplementary Material
%  Refined Inference for Asymptotically Linear Estimators
%  with Non-Negligible Second-Order Remainders
%  Submitted manuscript, May 2026
% ============================================================
\documentclass[12pt]{article}
\usepackage[margin=1in]{geometry}
\usepackage{amsmath,amssymb,amsthm}
\usepackage{mathtools}
\usepackage{booktabs}
\usepackage{array}
\usepackage{setspace}
\usepackage{parskip}
\usepackage{natbib}
\usepackage{hyperref}
\usepackage{doi}
\usepackage{enumitem}
\usepackage{caption}
\onehalfspacing

% ── Theorem environments (S-prefixed counters) ────────────────────────────────
\newtheorem{stheorem}{Theorem}[section]
\newtheorem{sproposition}[stheorem]{Proposition}

\newtheorem{sremark}{Remark}[section]

% ── Notation (must match main paper) ─────────────────────────────────────────
\newcommand{\EE}{\mathbb{E}}

\newcommand{\Psihat}{\hat{\Psi}}
\newcommand{\Psitrue}{\Psi(P_0)}

\newcommand{\Rrem}{R_{\mathrm{rem}}}
\newcommand{\sigEIF}{\sigma^2_{\mathrm{EIF}}}
\newcommand{\VarSand}{\widehat{\mathrm{Var}}_{\mathrm{Sand}}}
\newcommand{\VarJK}{\widehat{\mathrm{Var}}_{\mathrm{JK}}}
\newcommand{\VarBoot}{\widehat{\mathrm{Var}}_{\mathrm{Boot}}}

% ── Cross-references to main paper equations (reproduced for self-containment) ─
% eq:loo_lin from main paper Assumption 5.1:
%   max_i |n b_i + psi_{n,i}| -> 0
% Referenced below by name only

\begin{document}

\begin{center}
{\large\textbf{Supplementary Material}}\\[0.5em]
{\normalsize ``Refined Inference for Asymptotically Linear Estimators
with Non-Negligible Second-Order Remainders''}\\[0.3em]
{\normalsize \textit{Submitted manuscript}, May 2026}\\[0.3em]
{\normalsize \textit{Author information redacted for blind review}}
\end{center}

\medskip
\noindent This supplement collects technical conditions for the leave-one-out expansion, omitted proofs for the bootstrap and jackknife results, and an additional simulation illustrating the strong-decay regime. Section, theorem, proposition, and assumption numbers refer to the main paper.

\begin{itemize}[noitemsep]
  \item[\textbf{S1.}] Sufficient conditions for Assumption~5.1 (LOO Remainder Linearization)
  \item[\textbf{S2.}] Full proof of Theorem~5.2 (Bootstrap Variance Consistency)
  \item[\textbf{S3.}] Full proof of Theorem~5.4 (Jackknife Wald Interval Validity)
  \item[\textbf{S4.}] Secondary simulation: strong-decay regime (AIPW)
\end{itemize}

% ═══════════════════════════════════════════════════════════════════════════════
\section{Sufficient Conditions for Assumption~5.1}

Assumption~5.1 (LOO Remainder Linearization) requires a uniform linearization
$\max_i|nb_i + \psi_{n,i}|\xrightarrow{P}0$ with moment conditions (i)--(iii).
Controlling the leave-one-out perturbations $b_i = \Rrem^{(-i)} - \Rrem$
\emph{uniformly over all $n$ indices} is the key analytical task.  This is
structurally different from standard empirical process results, which control
$\Rrem(P_n)$ as a functional of the full empirical measure; the LOO perturbation
involves removing one observation from the nuisance training data, and uniform
control over $i$ requires a separate one-point-contamination argument.

\subsection*{S1.1\; Regular plug-in learners}

\begin{sproposition}[Smooth plug-in sufficient condition]
\label{sprop:hadamard}
Suppose:
\begin{enumerate}[label=\emph{(\roman*)}]
  \item \emph{(Differentiability.)}
    $P \mapsto \Rrem(P)$ is Hadamard differentiable at $P_0$
    with derivative $\dot\Rrem_{P_0}[\nu] = \int \psi \, d\nu$
    for some $\psi \in L^2_0(P_0)$ with $\mathrm{Var}(\psi)=c_R$
    and $\EE[\psi^4]<\infty$.
  \item \emph{(Uniform LOO expansion.)}
    $\sup_{1\le i\le n}|n(\Rrem^{(-i)}-\Rrem)+\psi(O_i)|\xrightarrow{P}0$.
\end{enumerate}
Then Assumption~5.1 holds with $\psi_{n,i}=\psi(O_i)$: conditions (i)--(iii)
follow from the LLN, $n^{-1}\sum_i\psi(O_i)^2\xrightarrow{P}c_R$, and
$n^{-1}\EE[\max_i\psi(O_i)^2]\le n^{-1}\sum_i\EE[\psi(O_i)^2]=c_R+o(1)<\infty$
and $\sup_i\EE[\psi(O_i)^4]<\infty$ by hypothesis, so condition~(iii) holds.
\end{sproposition}

\begin{sremark}[The two conditions are distinct]
Condition~(i) is a standard semiparametric differentiability requirement
that identifies $\psi$ and gives the structural interpretation of $c_R$.
Condition~(ii) is the non-trivial step: uniform control over $n$ LOO
perturbations simultaneously is not implied by Hadamard differentiability
alone.  It requires a one-point-contamination argument applied to the
composition of the nuisance maps and the remainder functional.

For bilinear remainders
$\Rrem=\int(\hat\eta_1-\eta_1^0)(\hat\eta_2-\eta_2^0)\,dP_0$,
Condition~(ii) can be established under additional one-point-contamination
regularity: both $P\mapsto\hat\eta_k(P)$ are Hadamard differentiable
at $P_0$, and the LOO stability condition
$\max_i\|\hat\eta_k^{(-i)}-\hat\eta_k\|_{P_0}=O_P(n^{-1/2})$ holds.
This provides a sufficient regular plug-in regime; a full general
verification theorem is not pursued here.
Under these conditions, a one-point-contamination expansion via the
chain rule for Hadamard derivatives
\citep[cf.][Chapter~20]{van_der_vaart1998asymptotic}
gives the uniform LOO linearization.
This regime covers fixed-weight ensembles and smooth sieves;
establishing Condition~(ii) for complex data-adaptive procedures
requires further case-specific analysis.
\end{sremark}

\subsection*{S1.2\; Data-adaptive learners}

\begin{sremark}[Data-adaptive case]
For learners that are not Hadamard differentiable, Condition~(ii) of
Proposition~S1.1 requires alternative verification.  Under a uniform
bounded-differences stability condition
$\sup_x|\hat\eta_k(\mathcal{D}_n;x)-\hat\eta_k(\mathcal{D}_n^{(-i)};x)|
= O(n^{-1})$ a.s., the bilinear structure of $\Rrem$ gives
$\max_i|nb_i|=O(r_n)\to 0$.
This stability route corresponds most naturally to regimes where
LOO perturbations are negligible --- consistent with the strong-decay
case ($c_R=0$) rather than a regime of non-negligible remainder variance.
In the near-boundary regime ($c_R>0$), the moment conditions of
Assumption~5.1 require additional learner-specific analysis beyond
uniform stability bounds.  Assumption~5.1 is stated as a direct condition
on the LOO perturbations to accommodate such case-by-case verification
without imposing a specific learner architecture.
\end{sremark}

\section{Full Proof of Theorem~5.2 (Bootstrap Variance Consistency)}
% ═══════════════════════════════════════════════════════════════════════════════

\begin{stheorem}[Bootstrap Variance Consistency]
Under Assumptions~2.1--2.4 of the main paper and Assumption~5.2 (Mallows--2 Bootstrap Consistency) of the main paper, the pairs bootstrap
variance satisfies $n\VarBoot \xrightarrow{P} \sigEIF + c_R$, where
$c_R = \lim_n n\cdot\mathrm{Var}(\Rrem)$ in the near-boundary regime
and $c_R = 0$ in the strong-decay regime.
\end{stheorem}

\begin{proof}
\textit{Step 1: Oracle bootstrap variance.}
Let $T_n = \sqrt{n}(\Psihat-\Psitrue)$ and $T_n^* = \sqrt{n}(\hat\Psi^*-\Psihat)$
be the centred bootstrap statistic.  Define the \emph{oracle} bootstrap variance
$V_n^{\rm oracle} := \EE^*[(T_n^*)^2\mid\mathcal{D}_n]$, the exact conditional
second moment of $T_n^*$ given the observed data.

By Assumption~5.2(ii), $d_2(T_n^*,T_n)\xrightarrow{P}0$, where $d_2$ is the
Wasserstein-2 distance.  Since Wasserstein-2 convergence is equivalent to weak
convergence plus convergence of second moments \citep{bickel1981some}:
\begin{equation}
  V_n^{\rm oracle}
  = \EE^*[(T_n^*)^2\mid\mathcal{D}_n]
  \;\xrightarrow{P}\; \EE[T_n^2]
  = \mathrm{Var}(T_n).
  \label{eq:oracle_conv}
\end{equation}
The target $\mathrm{Var}(T_n)=\sigEIF+c_R+o(1)$ follows from the variance
decomposition of Theorem~3.1:
$\mathrm{Var}(T_n)=\sigEIF + n\mathrm{Var}(\Rrem)+2n\mathrm{Cov}(\bar D_n,\Rrem)$,
with the cross term vanishing by Lemma~3.2 and $n\mathrm{Var}(\Rrem)\to c_R$.

\textit{Step 2: Oracle equals Monte Carlo in the $B\to\infty$ limit.}
The bootstrap variance estimator $\VarBoot(\Psihat)$ is defined as
the sample variance of $B$ i.i.d.\ bootstrap replicates
$\hat\Psi^{*1},\ldots,\hat\Psi^{*B}$:
\[
  \VarBoot(\Psihat)
  = \frac{1}{B}\sum_{b=1}^B
    \bigl(\hat\Psi^{*b}-\bar\Psi^*\bigr)^2,
  \quad
  \bar\Psi^* = \frac{1}{B}\sum_{b=1}^B\hat\Psi^{*b}.
\]
By the law of large numbers applied conditionally on $\mathcal{D}_n$,
as $B\to\infty$:
\[
  n\VarBoot(\Psihat)
  \;\xrightarrow{a.s.\mid\mathcal{D}_n}\;
  n\,\mathrm{Var}^*(T_n^*\mid\mathcal{D}_n)
  = V_n^{\rm oracle} - (\EE^*[T_n^*\mid\mathcal{D}_n])^2.
\]
By the LOO expansion of Lemma~4.1 in the main paper,
$\EE^*[\hat\Psi^*\mid\mathcal{D}_n] - \Psihat = O_P(n^{-1})$,
so the squared-mean correction
$(\EE^*[T_n^*\mid\mathcal{D}_n])^2 = n(\EE^*[\hat\Psi^*\mid\mathcal{D}_n]-\Psihat)^2
= O_P(n^{-1}) \xrightarrow{P} 0$.
Combined with \eqref{eq:oracle_conv}:
\[
  n\VarBoot(\Psihat) \;\xrightarrow{P}\; \sigEIF + c_R.
\]
Condition~(i) of Assumption~5.2 ($\sup_n\EE[T_n^2]<\infty$) holds since
$\sigEIF+c_R+o(1)$ is bounded.
\end{proof}

% ═══════════════════════════════════════════════════════════════════════════════
\section{Full Proof of Theorem~5.4 (Jackknife Wald Interval Validity)}
% ═══════════════════════════════════════════════════════════════════════════════

\begin{stheorem}[Jackknife Wald Interval Validity]
Under the conditions of Theorems~5.1 (Jackknife Variance Consistency)
and~5.3 (Bootstrap Wald Interval Validity),
the studentized jackknife pivot
$T_n^{\rm JK} = \sqrt{n}(\Psihat - \Psitrue)/\sqrt{n\VarJK} \Rightarrow N(0,1)$,
and the jackknife Wald interval achieves asymptotically exact coverage.
\end{stheorem}

\begin{proof}
\textit{Step 1: Bootstrap pivot validity.}
By Theorem~5.3 (Bootstrap Wald Interval Validity) and Assumption~7
(Near-Boundary CLT), the bootstrap Wald pivot satisfies
$\sqrt{n}(\Psihat - \Psitrue)/\sqrt{n\VarBoot} \Rightarrow N(0,1)$.

\textit{Step 2: Ratio convergence.}
By Theorem~5.1, $n\VarJK \xrightarrow{P} \sigEIF + c_R$.
By Theorem~5.2, $n\VarBoot \xrightarrow{P} \sigEIF + c_R$.
Therefore $\VarJK/\VarBoot \xrightarrow{P} 1$.

\textit{Step 3: Transfer of validity.}
Write
\[
  T_n^{\rm JK}
  = \frac{\sqrt{n}(\Psihat-\Psitrue)}{\sqrt{n\VarBoot}}
    \cdot \sqrt{\frac{\VarBoot}{\VarJK}}.
\]
The first factor converges in distribution to $N(0,1)$ (Step~1).
The second factor converges in probability to $1$ (Step~2).
Both quantities are measurable functions of the same data $\mathcal{D}_n$,
so Slutsky's theorem gives $T_n^{\rm JK}\Rightarrow N(0,1)$.

\textit{Strong-decay regime ($c_R = 0$).}
Both $n\VarJK$ and $n\VarBoot$ converge to $\sigEIF$;
the argument is identical.
\end{proof}

% ═══════════════════════════════════════════════════════════════════════════════
\section{Secondary Simulation: Strong-Decay Regime (AIPW)}
% ═══════════════════════════════════════════════════════════════════════════════

This section illustrates the strong-decay regime using a non-cross-fitted
augmented inverse probability weighted (AIPW) estimator in an i.i.d.\
observational study.  The purpose is to demonstrate that the variance ratio
$\hat\rho = \VarJK/\VarSand$ decreases to $1.0$ as $n$ grows when nuisance
estimation operates in the strong-decay regime
($n\cdot\mathrm{Var}(\Rrem)\to 0$), in contrast to the persistent
near-boundary behaviour of Table~1 in the main paper.

\subsection*{S4.1\; Data-generating process}

\begin{alignat*}{3}
  W &\sim N(0,1), \quad
  &A \mid W &\sim \mathrm{Bernoulli}(\mathrm{expit}(0.3W)),\\
  Y &= 0.5 + 0.4A + 0.3W + 0.15AW + \varepsilon, \quad
  &\varepsilon &\sim N(0, 0.5^2).
\end{alignat*}
True ATE: $\Psi_0 = 0.4$.  Nuisance models: outcome regression correctly
specified as $\mathrm{lm}(Y \sim A \times W)$; propensity enriched as
$\mathrm{glm}(A \sim W + W^2)$.  No cross-fitting ($V=1$) ensures the
full-data and leave-one-out fits are structurally comparable.  Under
correctly specified parametric nuisance at $O_P(n^{-1/2})$ convergence,
$n\cdot\mathrm{Var}(\Rrem)\to 0$, placing the estimator in the strong-decay
regime (Theorem~4.1 of the main paper).

\subsection*{S4.2\; Results}

\begin{table}[h]
\centering
\caption{AIPW secondary simulation: strong-decay regime.
  $\hat\rho = \bar{V}_{\rm JK}/\bar{V}_{\rm Sand}$ decreases monotonically
  to $1.0$, confirming $n\cdot\mathrm{Var}(\Rrem)\to 0$ under $O_P(n^{-1/2})$
  parametric nuisance.
  CP(Sand) and CP(JK): empirical 95\% CI coverage ($z_{\alpha/2}$ critical values).
  $R = 500$ replicates; MC-SE $\approx 0.010$.}
\label{tab:aipw}
\smallskip
\begin{tabular}{crrrrrr}
\toprule
$n$ & Bias & MCSD & CP(Sand) & CP(JK) & $\hat\rho$ \\
\midrule
 200 & $+0.000$ & $0.070$ & $0.964$ & $0.968$ & $1.040$ \\
 500 & $-0.002$ & $0.045$ & $0.946$ & $0.946$ & $1.014$ \\
1000 & $-0.001$ & $0.031$ & $0.960$ & $0.960$ & $1.007$ \\
2000 & $-0.000$ & $0.023$ & $0.958$ & $0.958$ & $1.003$ \\
\bottomrule
\end{tabular}
\end{table}

$\hat\rho$ decreases monotonically from $1.040$ to $1.003$, consistent
with the sharp sandwich characterization (Theorem~4.1 of the main paper):
under $O_P(n^{-1/2})$ nuisance convergence, $n\VarSand \xrightarrow{P} \sigEIF$
and $n\VarJK \xrightarrow{P} \sigEIF$, so no correction beyond the sandwich
is needed.  All coverage probabilities lie within $\pm 2$ Monte Carlo
standard errors of $0.95$.  This contrasts with Table~1 of the main paper,
where $\hat\rho$ remains above $1.14$ across all $J$ under the structural near-boundary remainder in the primary running example.

\noindent\textit{Note on $V=1$.} No cross-fitting ensures the LOO and full-data
nuisance fits are structurally comparable.  Cross-fitting is standard in
practice but is not needed for the strong-decay conclusion.

% ── References ────────────────────────────────────────────────────────────────
\bibliographystyle{plainnat}
\bibliography{references}

\end{document}
